# Supplementary material for: ActionSwitch: Class-agnostic Detection of Simultaneous Actions in Streaming Videos
Source: arXiv:2407.12987 source file (2024-07-17)

a)

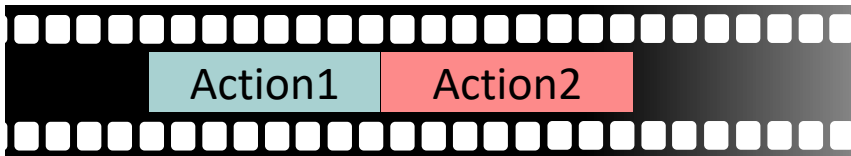

b)

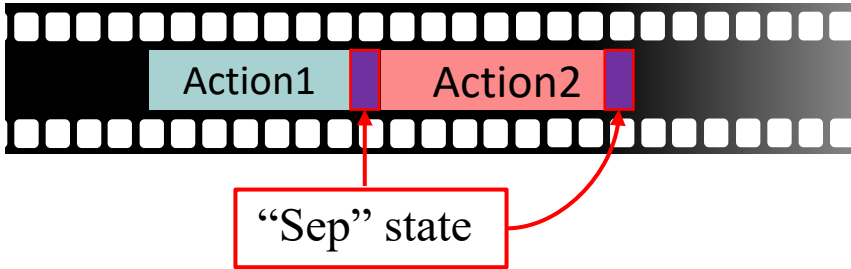

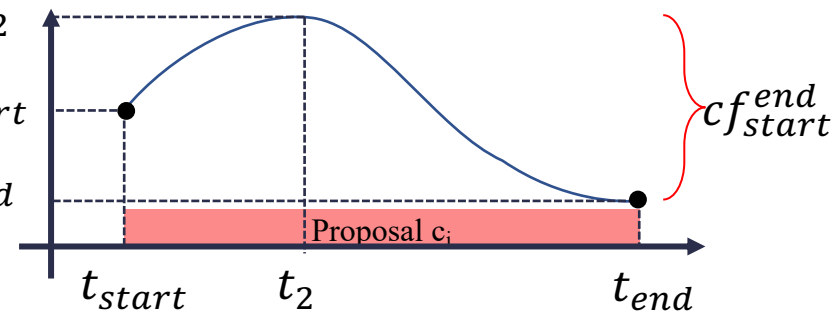

mAP metric:  $(t_{start}, t_{end}, c_i, c_{f_{end}})$

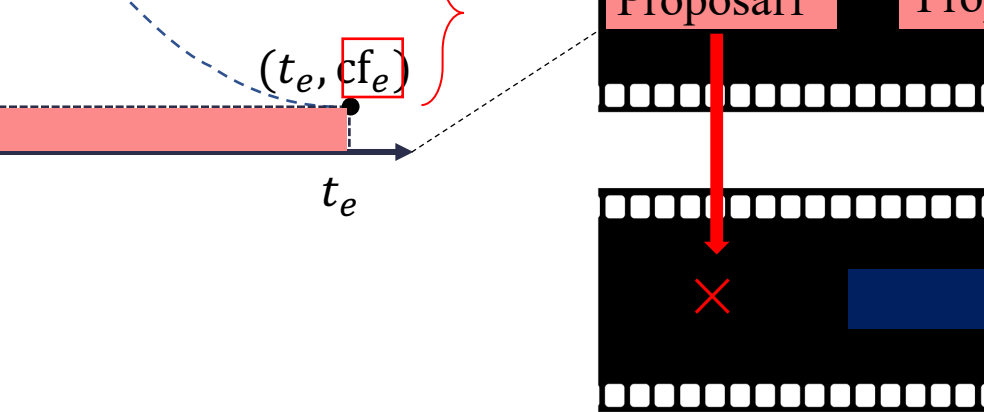

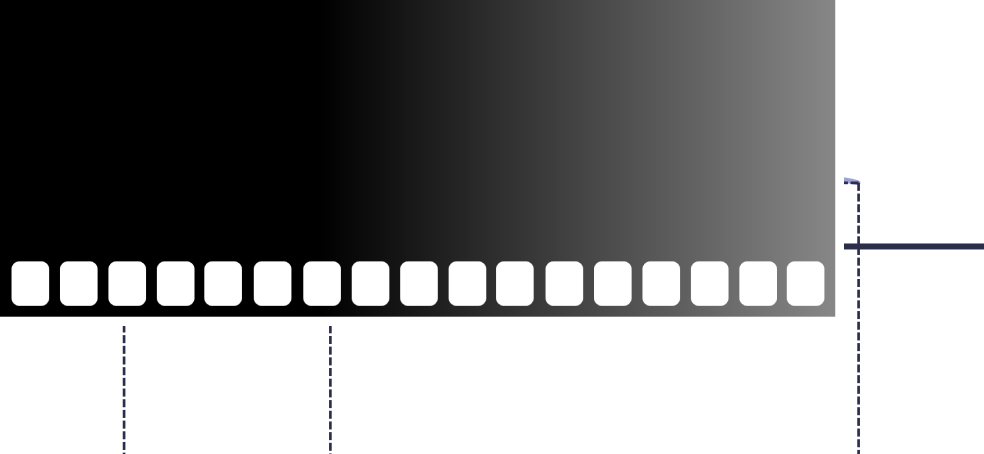

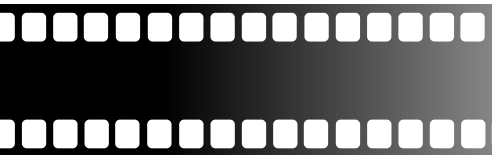

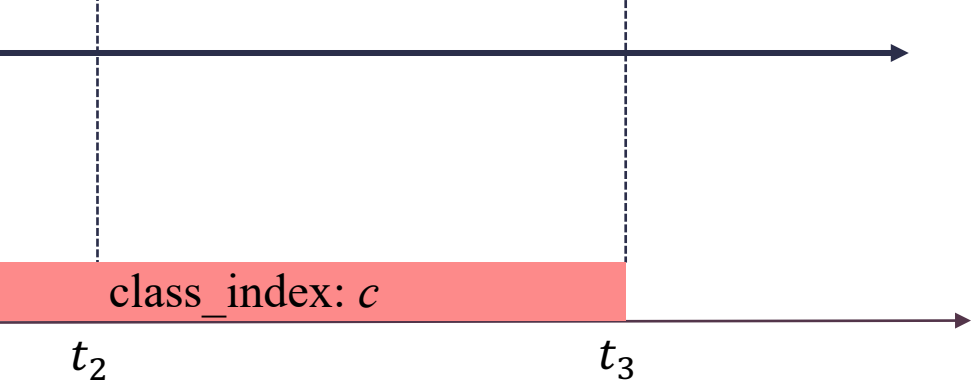

Supplement: Supplementary file 1 [file supple_fig2.pdf]
