# Supplementary material for: ActionSwitch: Class-agnostic Detection of Simultaneous Actions in Streaming Videos
Source: arXiv:2407.12987 source file (2024-07-17)
Supplement: Supplementary file 2 [file supplefig.pdf]

# Evaluation target

mAP metric:

$(t_s, t_e, c, \text{cf}_e)$

Hungarian F1 score:

$(t_s, t_e)$

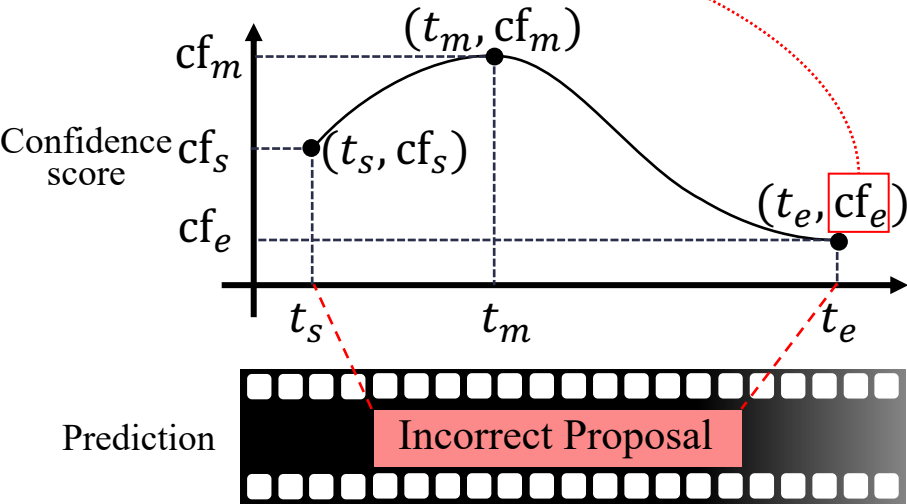

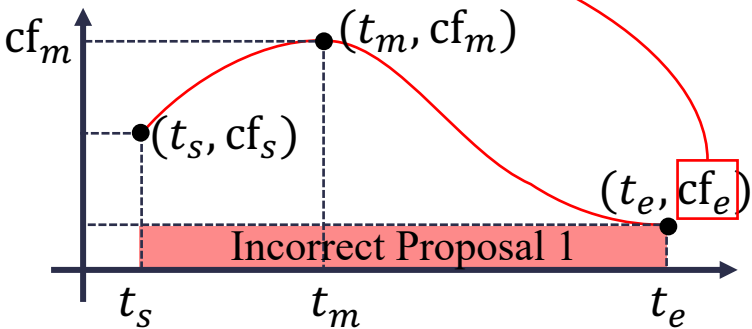

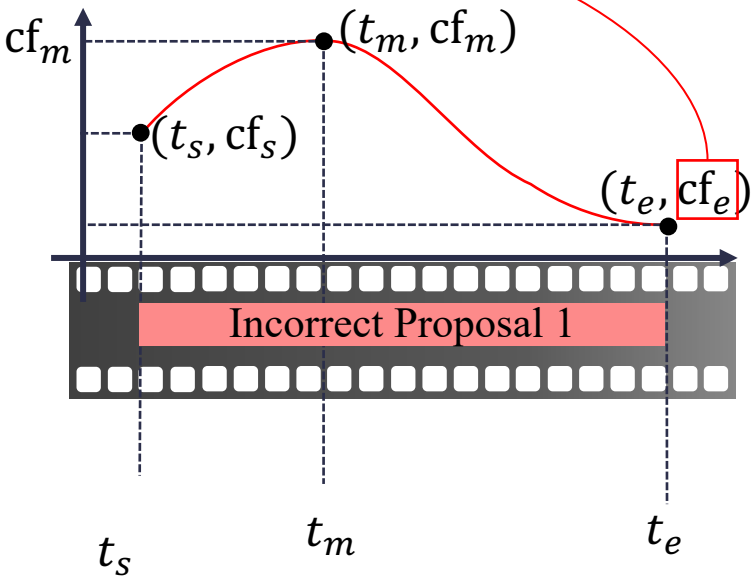



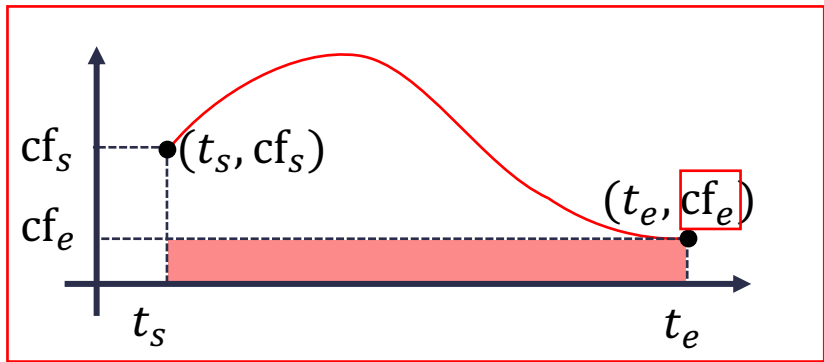

Proposal1

Proposal2
